# Supplementary material for: The interplay between strong correlation and adsorption distances
Source: arXiv:1710.07349 ancillary file (2017-12-21)
Supplement: Supplementary file 1 [file supplemental.pdf]

# Supplemental Material: The interplay between strong correlation and adsorption distances


Marc Philipp Bahlke and Carmen Herrmann
*Institut für Anorganische und Angewandte Chemie, Universität Hamburg, Martin-Luther-King-Platz 6, 20146 Hamburg, Germany*

Michael Karolak
*Institut für Theoretische Physik und Astrophysik, Universität Würzburg, Am Hubland, 97074 Würzburg, Germany*



(Dated: October 19, 2017)


## I. SUPPLEMENTAL MATERIAL

### A. Potential energy surface

Fig. 1 shows the PES as calculated with LDA++ and PBE++ with $U$ = 3.8 eV, 4.0 eV and 4.2 eV. For PBE++ there is no shift of the adsorption distance of Co on Cu(100), whereas for LDA++ the minimum shifts from 1.52 Å to 1.54 Å by increasing $U$ from 4.0 eV to 4.2 eV. The adsorption distance of LDA++ does not further increase upon increasing $U$ from 4.2 eV to 5.0 eV (see Fig. 2, but note that the abscissa is reduced compared to Fig. 1).

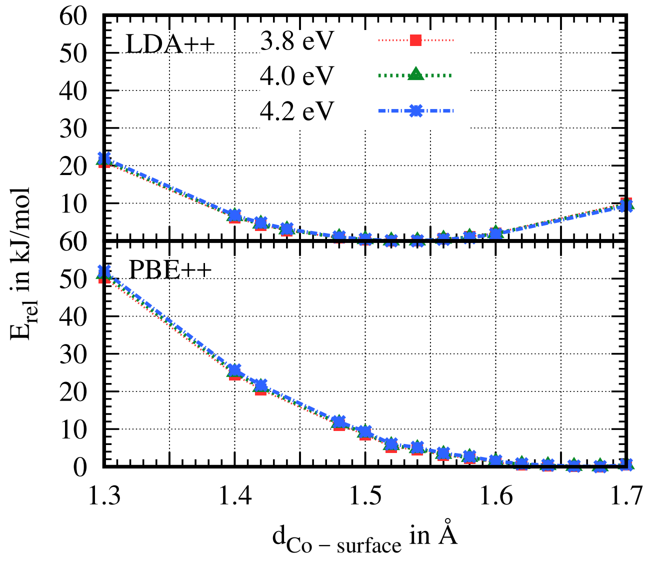


FIG. 1. Relative energies as obtained from DFT++ for different adsorption distances of Co on Cu(100). The DFT++ calculations were performed at $\beta = 100$ eV$^{-1}$. The DFT++ results for $U$ = 3.8 eV, 4.0 eV and 4.2 eV are nearly on top of each other. The exchange parameter for all values of $U$ is $J = 0.9$ eV.

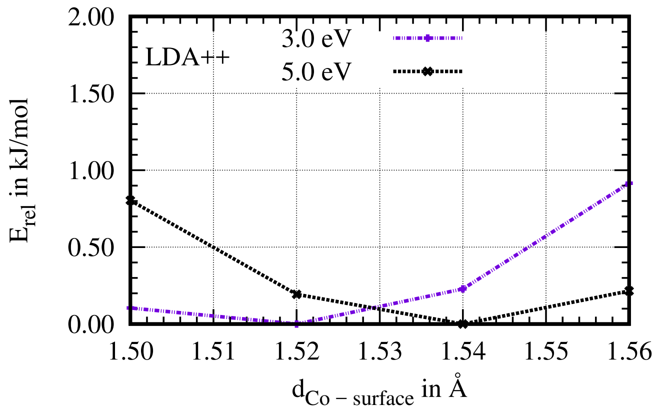


FIG. 2. Relative energies as obtained from LDA++ for different adsorption distances of Co on Cu(100). The LDA++ calculations were performed at $\beta = 100$ eV$^{-1}$ for $U = 3.0$ eV and 5.0 eV, both with $J = 0.9$ eV.

## B. Hybridization functions

In Fig. 3, the hybridization function of Co on Cu(100) as obtained from PBE is shown for selected values of $d_{\mathrm{Co-surface}}$. By comparison with Fig. 6 of the main article, one can notice that both functionals (LDA and PBE) yield a similar hybridization function at all adsorption distances shown here.
Fig. 4 shows the real part of the hybridization function of Co on Cu(100) at 1.30 Å and 1.70 Å as obtained from LDA. The real part of the hybridization function can be seen as the energy/frequency dependent shift of the impurity level. By comparing Fig. 4 a) and b), one can see that the shift of the impurity levels as a function of the energy is larger if Co is closer to the Cu(100) surface.

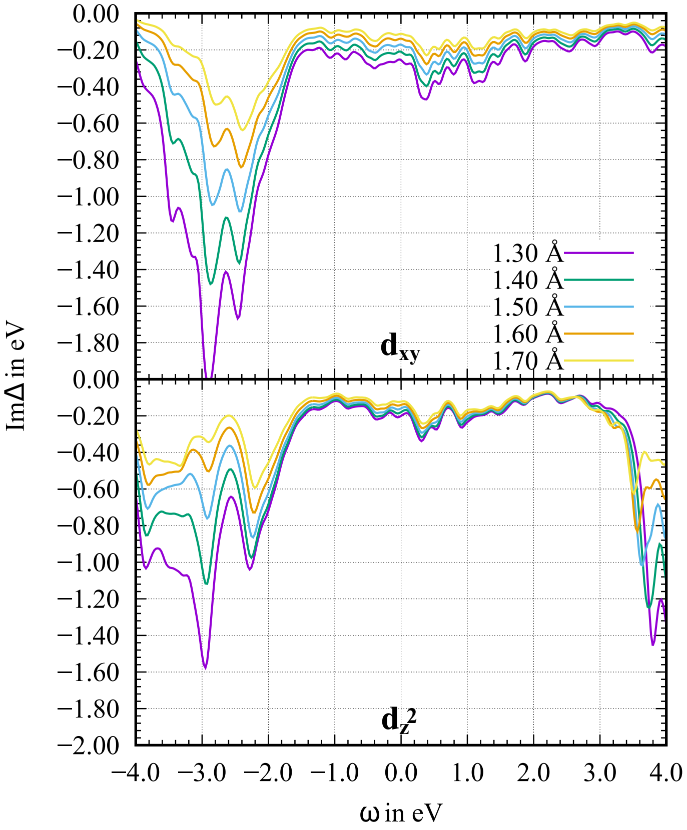


FIG. 3. Imaginary part of the hybridization function for the Co $3d_{xy}$ and the Co $3d_{z^2}$ orbital as obtained from PBE, for selected values of $d_{\mathrm{Co-surface}}$.

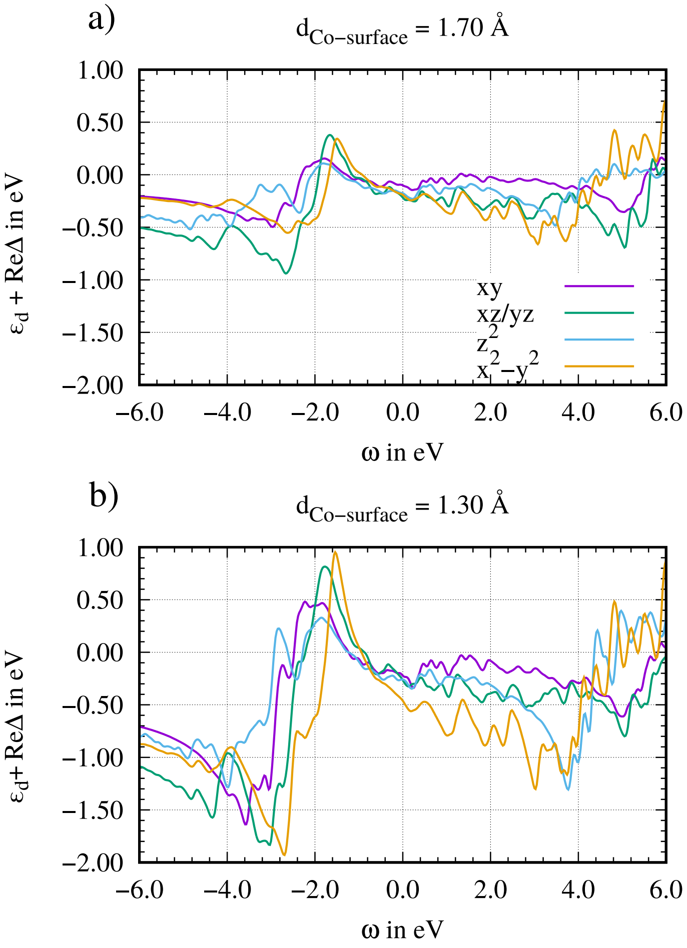


FIG. 4. Real part of the hybridization function of all Co 3$d$ orbitals at $d_{\text{Co-surface}} = 1.70$ Å and 1.30 Å. Results are obtained from LDA.

### C. Self-energies

In Fig. 5 we provide ImΣ as obtained from DFT++ ($U = 4.0$ eV and $J = 0.9$ eV at $\beta = 100^{-1}$ eV) at selected values for the adsorption distances for the Co $3d_{xz/yz}$ and the $3d_{x^2-y^2}$ orbital. Note that in contrast to Fig. 7 of the main article the abscissa in Fig.5 is reduced.

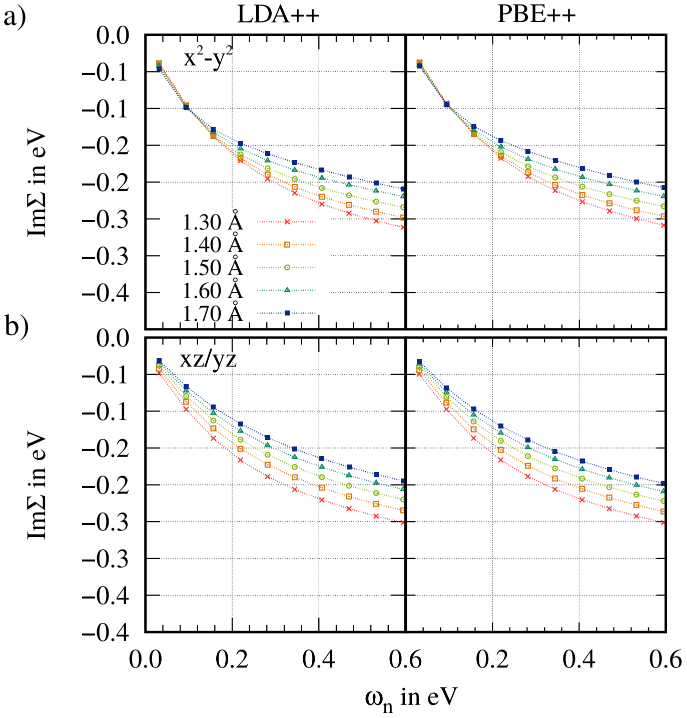


FIG. 5. Self energies obtained from DFT++ at $\beta = 100$ eV$^{-1}$ with $U = 4.0$ eV and $J = 0.9$ eV. a) ImΣ for the Co $3d_{x^2-y^2}$ orbital as obtained from LDA++ and PBE++. b) ImΣ for the Co $3d_{xz/yz}$ orbital as obtained from LDA++ and PBE++.

### D. PBE results

In Fig. 6 the Co $3d$ crystal-field splitting as a function of the adsorption distance is shown, as obtained from PBE. Comparison with Fig. (5) of the main article shows that both functionals predict a similar crystal-field splitting at all adsorption distances under study here.

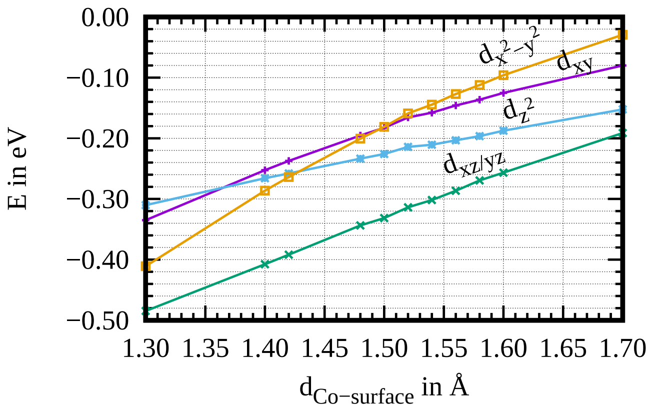


FIG. 6. Static crystal-field splitting (*i.e.* $3d$-orbital energies of Co) of the Co $3d$ shell as obtained from PBE (spin-unpolarized), as a function of the adsorption distance. The Fermi level is set to zero.

In Tab. I we provide the estimated Kondo temperatures as obtained from Eq. (15) of the main article. For $\epsilon_{xy/z^2}$ and Im$\Delta_{xy,z^2}$ we used the values as obtained from spin-unpolarized PBE.

TABLE I. Estimated Kondo temperature as obtained from a one-band model with a constant hybridization. Im$\Delta(0)$ is the value of the imaginary part of the hybridization function at $\omega = 0$ eV (Fermi level). $\epsilon_{xy/z^2}$ are the energies of the Co $d_{xy/z^2}$ orbitals related to the Fermi level. Values taken here are obtained from PBE, and for $U$ we have chosen 4.0 eV. For the estimation of the Kondo temperature $T_{\mathrm{K}}$ see Eq. (15) of the main article. Experimental value for $T_{\mathrm{K}} = 88 \pm 4$ K$^{1-3}$.

| $d_{\mathrm{Co-surf.}}$ | -Im$\Delta_{xy}(0)$ | -Im$\Delta_{z^2}(0)$ | $\epsilon_{xy}$ | $\epsilon_{z^2}$ | $T_{\mathrm{K},xy}$ | $T_{\mathrm{K},z^2}$ |
|---|---|---|---|---|---|---|
| 1.30 Å | 0.255 | 0.200 | -0.335 | -0.310 | 133.4 | 58.55 |
| 1.40 Å | 0.210 | 0.180 | -0.253 | -0.266 | 153.4 | 63.95 |
| 1.50 Å | 0.171 | 0.159 | -0.183 | -0.226 | 195.0 | 69.52 |
| 1.60 Å | 0.139 | 0.140 | -0.125 | -0.187 | 276.2 | 79.54 |
| 1.70 Å | 0.112 | 0.122 | -0.080 | -0.152 | 428.0 | 94.00 |

### E. Configuration- and spin state probabilities

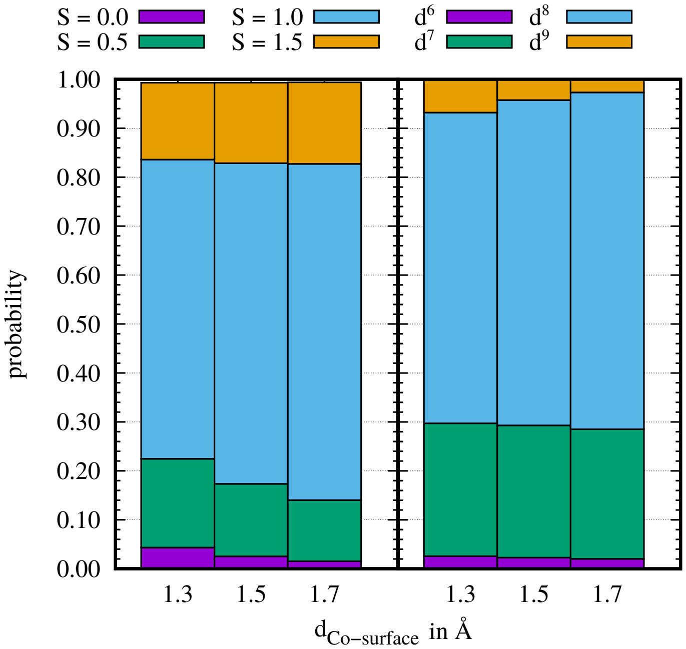


FIG. 7. Most probable spin staes ($S$) and atomic configuration as obtained from LDA++ for Co/Cu(001) for selected values of $d_{\mathrm{Co-surface}}$. The LDA++ calculations were performed at $\beta$ = 100 eV $^{-1}$, $U$ = 4.0 eV abd $J$ = 0.9 eV.

From Fig. 7 one can see that at all adsorption distances under study here the Co atom is predominantly in a $d^8$, $S$=1 configuration. The character of these configuration slightly increases for larger adsorption distances.

### F. Specification of the unit cell

In Tab. II we provide the coordinates of all atoms in the unit cell used in our calculations. Note that the Cu atoms were kept frozen, and only the Co $z$-coordinate was varied between 1.30 Å and 1.70 Å.

TABLE II. $xyz$-coordinates of all atoms contained in the unit cell with $d_{\mathrm{Co-surface}} = 1.30$ Å. Values are given in Å.

| Atom | $x$-coord. | $y$-coord. | $z$-coord. | Atom | $x$-coord. | $y$-coord. | $z$-coord. |
|---|---|---|---|---|---|---|---|
| Cu | 1.807445 | 9.037225 | -7.229780 | Cu | 3.614890 | 5.422335 | -1.807445 |
| Cu | 0.000000 | 7.229780 | -7.229780 | Cu | 5.422335 | 5.422335 | 0.000000 |
| Cu | 0.000000 | 9.037225 | -5.422335 | Cu | 3.614890 | 3.614890 | 0.000000 |
| Cu | 1.807445 | 9.037225 | -3.614890 | Cu | 5.422335 | 3.614890 | -1.807445 |
| Cu | 0.000000 | 7.229780 | -3.614890 | Cu | 9.037225 | 5.422335 | -7.229780 |
| Cu | 1.807445 | 7.229780 | -5.422335 | Cu | 7.229780 | 3.614890 | -7.229780 |
| Cu | 0.000000 | 9.037225 | -1.807445 | Cu | 7.229780 | 5.422335 | -5.422335 |
| Cu | 1.807445 | 9.037225 | 0.000000 | Cu | 9.037225 | 5.422335 | -3.614890 |
| Cu | 0.000000 | 7.229780 | 0.000000 | Cu | 7.229780 | 3.614890 | -3.614890 |
| Cu | 1.807445 | 7.229780 | -1.807445 | Cu | 9.037225 | 3.614890 | -5.422335 |
| Cu | 5.422335 | 9.037225 | -7.229780 | Cu | 7.229780 | 5.422335 | -1.807445 |
| Cu | 3.614890 | 7.229780 | -7.229780 | Cu | 9.037225 | 5.422335 | 0.000000 |
| Cu | 3.614890 | 9.037225 | -5.422335 | Cu | 7.229780 | 3.614890 | 0.000000 |
| Cu | 5.422335 | 9.037225 | -3.614890 | Cu | 9.037225 | 3.614890 | -1.807445 |
| Cu | 3.614890 | 7.229780 | -3.614890 | Cu | 1.807445 | 1.807445 | -7.229780 |
| Cu | 5.422335 | 7.229780 | -5.422335 | Cu | 0.000000 | 0.000000 | -7.229780 |
| Cu | 3.614890 | 9.037225 | -1.807445 | Cu | 0.000000 | 1.807445 | -5.422335 |
| Cu | 5.422335 | 9.037225 | 0.000000 | Cu | 1.807445 | 1.807445 | -3.614890 |
| Cu | 3.614890 | 7.229780 | 0.000000 | Cu | 0.000000 | 0.000000 | -3.614890 |
| Cu | 5.422335 | 7.229780 | -1.807445 | Cu | 1.807445 | -0.000000 | -5.422335 |
| Cu | 9.037225 | 9.037225 | -7.229780 | Cu | 0.000000 | 1.807445 | -1.807445 |
| Cu | 7.229780 | 7.229780 | -7.229780 | Cu | 1.807445 | 1.807445 | 0.000000 |
| Cu | 7.229780 | 9.037225 | -5.422335 | Cu | 0.000000 | 0.000000 | 0.000000 |
| Cu | 9.037225 | 9.037225 | -3.614890 | Cu | 1.807445 | -0.000000 | -1.807445 |
| Cu | 7.229780 | 7.229780 | -3.614890 | Cu | 5.422335 | 1.807445 | -7.229780 |
| Cu | 9.037225 | 7.229780 | -5.422335 | Cu | 3.614890 | -0.000000 | -7.229780 |
| Cu | 7.229780 | 9.037225 | -1.807445 | Cu | 3.614890 | 1.807445 | -5.422335 |
| Cu | 9.037225 | 9.037225 | 0.000000 | Cu | 5.422335 | 1.807445 | -3.614890 |
| Cu | 7.229780 | 7.229780 | 0.000000 | Cu | 3.614890 | -0.000000 | -3.614890 |
| Cu | 9.037225 | 7.229780 | -1.807445 | Cu | 5.422335 | -0.000000 | -5.422335 |
| Cu | 1.807445 | 5.422335 | -7.229780 | Cu | 3.614890 | 1.807445 | -1.807445 |
| Cu | 0.000000 | 3.614890 | -7.229780 | Cu | 5.422335 | 1.807445 | 0.000000 |
| Cu | 0.000000 | 5.422335 | -5.422335 | Cu | 3.614890 | -0.000000 | 0.000000 |
| Cu | 1.807445 | 5.422335 | -3.614890 | Cu | 5.422335 | -0.000000 | -1.807445 |
| Cu | 0.000000 | 3.614890 | -3.614890 | Cu | 9.037225 | 1.807445 | -7.229780 |
| Cu | 1.807445 | 3.614890 | -5.422335 | Cu | 7.229780 | -0.000000 | -7.229780 |
| Cu | 0.000000 | 5.422335 | -1.807445 | Cu | 7.229780 | 1.807445 | -5.422335 |
| Cu | 1.807445 | 5.422335 | 0.000000 | Cu | 9.037225 | 1.807445 | -3.614890 |
| Cu | 0.000000 | 3.614890 | 0.000000 | Cu | 7.229780 | -0.000000 | -3.614890 |
| Cu | 1.807445 | 3.614890 | -1.807445 | Cu | 9.037225 | -0.000000 | -5.422335 |
| Cu | 5.422335 | 5.422335 | -7.229780 | Cu | 7.229780 | 1.807445 | -1.807445 |
| Cu | 3.614890 | 3.614890 | -7.229780 | Cu | 9.037225 | 1.807445 | 0.000000 |
| Cu | 3.614890 | 5.422335 | -5.422335 | Cu | 7.229780 | -0.000000 | 0.000000 |
| Cu | 5.422335 | 5.422335 | -3.614890 | Cu | 9.037225 | -0.000000 | -1.807445 |
| Cu | 3.614890 | 3.614890 | -3.614890 | Co | 5.422335 | 3.614890 | 1.30 |
| Cu | 5.422335 | 3.614890 | -5.422335 | | | | |

[1] N. Knorr, M. A. Schneider, L. Diekhner, P. Wahl, and K. Kern, Phys. Rev. Lett. **88**, 096804 (2002).
[2] P. Wahl, L. Diekhner, M. A. Schneider, L. Vitali, G. Wittich, and K. Kern, Phys. Rev. Lett. **93**, 2004 (2004).
[3] P. Wahl, A. P. Seitsonen, L. Diekhner, M. A. Schneider, and K. Kern, New J. Phys. **11**, 2009 (2009).
